# Supplementary material for: Reliable Real Time Ball Tracking for Robot Table Tennis
Source: arXiv:1908.07332 source file (2019-08-20)
Supplement: Supplementary file 1 [file appendices.tex]

\section{Appendix if needed}

\begin{comment}
\section{Appendix Title Goes Here}
Appendix one text goes here.

% you can choose not to have a title for an appendix
% if you want by leaving the argument blank
\section{}
Appendix two text goes here.

% use section* for acknowledgment
\section*{Acknowledgment}

The authors would like to thank...
\end{comment}
